# Supplementary material for: Stopping narrow-band x-ray pulses in nuclear media
Source: arXiv:1508.06762 source file (2016-05-20)
Supplement: Supplementary file 1 [file SupplementaryMaterial.pdf]

# Stopping narrow-band x-ray pulses in nuclear media: Supplementary Material

Xiangjin Kong and Adriana Pálffy
Max-Planck-Institut für Kernphysik, Saupfercheckweg 1, 69117 Heidelberg, Germany

In the following we present in detail the analytic derivation of the expressions presented in the main text and discuss on the numerical parameters used.

## COLLECTIVE NUCLEAR STATES

We assume that the nuclei are initially in the collective ground state

$$|G\rangle = \underbrace{|g_1^{(1)}\rangle \dots |g_1^{(N_1)}\rangle}_{N_1} \underbrace{|g_2^{(N_1+1)}\rangle \dots |g_2^{(N)}\rangle}_{N_2}, \tag{S1}$$

where $|g_1\rangle$ and $|g_2\rangle$ denote the two ground magnetic sublevels and $N_i$ is the number of nuclei in the ground state $|g_i\rangle$ $(i \in 1,2)$, $N_1 + N_2 = N$ and $N_1 \approx N_2$ at room temperature.

Current experiments employing the 14.4 keV resonance line in $^{57}$Fe are mostly performed at modern synchrotron light sources. There is less than one resonant photon on average in each pulse. Thus, we assume that only one nucleus can be excited at a time and omit higher excited states. We consider in the following an x-ray pulse with incident polarization oriented with respect to the magnetic field such that only the two $\Delta m = 0$ transitions are driven. We define the excited state as a timed Dicke state

$$|E_\mu\rangle = \frac{1}{\sqrt{N_\mu}} \sum_n^{N_\mu} e^{i\vec{k}_C \cdot \vec{R}^{(n)}} |g_1^{(1)}\rangle \dots |e_\mu^{(n)}\rangle \dots |g_2^{(N)}\rangle, \tag{S2}$$

in which the $n$th atom has been excited by the transition $\mu$, with the notation $\mu = 1$ for the transition $m_g = -1/2 \to m_e = -1/2$ and $\mu = 2$ for $m_g = 1/2 \to m_e = 1/2$, depending on the initial ground state spin projection $m_g$. The position of the excited nucleus is given by $\vec{R}^{(n)}$ and $\vec{k}_C$ represents the total wave vector for the resonant cavity mode. The two $\Delta m = 0$ transitions are equivalent in this system to the two transitions $|3\rangle \to |1\rangle$ and $|3\rangle \to |2\rangle$, where we have used the notation $|3\rangle$ for $|G\rangle$, $|1\rangle$ for $|E_1\rangle$ and $|2\rangle$ for $|E_2\rangle$, respectively, as illustrated in the inset panel in Fig. 1 in the main text. The two transitions experience vacuum-mediated coupling by spontaneously generated coherence terms [43].

## DENSITY MATRIX FORMALISM

We use the master equation to describe the dynamics of the system [43]

$$\frac{d}{dt}\rho = -i[H_M + H_N, \rho] + L_M[\rho] + L_{SE}[\rho]. \tag{S3}$$

The Hamiltonian consists of two parts: one is the interaction between the incident pulse and the cavity $H_M$ and the other is the interaction between the cavity and the resonant nuclei $H_N$. Moreover, $L_M[\rho]$ accounts for the loss of the cavity and $L_{SE}[\rho]$ for the spontaneous emission, respectively. In the interaction picture, the Hamiltonian corresponding to the x-ray-cavity interaction can be written as follows [43]:

$$H_M = \Delta_c a_1^+ a_1 + \Delta_c a_2^+ a_2 + i\sqrt{2\kappa_R}[(\hat{a}_1^* \cdot \hat{a}_{in})a_{in}a_1^+ - (\hat{a}_{in}^* \cdot \hat{a}_1)a_{in}^* a_1 + (\hat{a}_2^* \cdot \hat{a}_{in})a_{in}a_2^+ - (\hat{a}_{in}^* \cdot \hat{a}_2)a_{in}^* a_2]. \tag{S4}$$

Here, $\Delta_c$ is the cavity detuning, $a$ ($a^+$) is the photon annihilation (creation) operator and $a_1$, $a_2$ represent the two different modes defined according to the polarization state of the photon. Furthermore, $\kappa_R$ denotes the x-ray coupling strength into the cavity mode, and $a_{in}$ characterizes the driving field of the cavity mode by the external (classical) x-ray field. The products $(\hat{a}_i^* \cdot \hat{a}_j)$ are scalar products between two different polarization unit vectors.

On the other hand, the cavity-nucleus interaction Hamiltonian reads

$$\begin{aligned} H_N &= -\Delta \sum_\mu |E_\mu\rangle\langle E_\mu| - \sum_\mu \Delta_\mu |E_\mu\rangle\langle E_\mu| \\ &+ \sum_{j=1}^{2}\sum_\mu \left[(\hat{d}_\mu^* \cdot \hat{a}_j)c_\mu \sqrt{N_\mu} g |E_\mu\rangle\langle G| a_j + (\hat{a}_j^* \cdot \hat{d}_\mu)c_\mu \sqrt{N_\mu} g^* a_j^+ |G\rangle\langle E_\mu|\right]. \end{aligned} \tag{S5}$$

In the expression above, $\Delta$ is the detuning between the x-ray field and the bare transition energy of the nuclei, and $\Delta_\mu$ is the energy difference induced by the hyperfine splitting. The normalized dipole moment $\hat{d}_\mu$ of transition $\mu$ is defined with respect of the axis of nuclei, i.e., the orientation of the magnetic hyperfine field $\hat{B}$. Furthermore, $g$ is the coupling strength between the ensemble and the cavity and $c_\mu$ denotes the corresponding Clebsch-Gordan coefficient.

The thin film cavity considered in this work has a low quality factor which means the decay rate of the cavity $\kappa$ is much larger than the atom-field coupling strength $g$. Thus, we can eliminate the cavity modes adiabatically, i.e., we set $\frac{d}{dt}a_j = 0$ . The Heisenberg equation of motion for the operator $a_j$ then reads

$$\frac{d}{dt}a_j = i[H_M + H_N, a_j] - \kappa a_j = 0. \tag{S6}$$

Introducing the expressions (S4) and (S5) into Eq. (S6), we obtain

$$a_j = \frac{\sqrt{2k_R}(\hat{a}_j^{*}\cdot\hat{a}_{in})a_{in} - i\sum_\mu(\hat{a}_j^{*}\cdot\hat{d}_\mu)c_\mu\sqrt{N_\mu}g^{*}|G\rangle\langle E_\mu|}{\kappa + i\Delta_c}\,. \tag{S7}$$

Inserting the expression (S7) into the Hamiltonian terms (S4) and (S5), we can obtain the master equation (S3) in another form (see also [43])

$$\frac{d}{dt}\rho = -i[H_0 + H_\Omega + H_{LS}, \rho] + L_{cav}[\rho]\,, \tag{S8}$$

with the following notations

$$\begin{aligned}
H_0 &= -\Delta\sum_\mu|E_\mu\rangle\langle E_\mu| - \sum_\mu\Delta_\mu|E_\mu\rangle\langle E_\mu|\,,\\
H_\Omega &= \Omega\sum_\mu(\hat{d}_\mu^{*}\cdot\mathbb{1}_\perp\cdot\hat{a}_{in})c_\mu\sqrt{N_\mu}g|E_\mu\rangle\langle G| + H.c.\,,\\
H_{LS} &= \delta_{LS}\sum_{\mu,\nu}(\hat{d}_\mu^{*}\cdot\mathbb{1}_\perp\cdot\hat{d}_\nu)c_\mu c_\nu|g|^2\sqrt{N_\mu N_\nu}|E_\mu\rangle\langle E_\nu|\,,\\
L_{cav}[\rho] &= -\zeta_S\sum_{\mu,\nu}(\hat{d}_\mu^{*}\cdot\mathbb{1}_\perp\cdot\hat{d}_\nu)c_\mu c_\nu|g|^2\sqrt{N_\mu N_\nu}L[\rho, |E_\mu\rangle\langle G|, |G\rangle\langle E_\nu|]\,.
\end{aligned} \tag{S9}$$

Here, $\mathbb{1}_\perp = \hat{a}_1\hat{a}_1^{*} + \hat{a}_2\hat{a}_2^{*}$ with the mode operators connected by an outer product rather than a scalar product. The transition dipole moments are thus not coupled to the polarization of the external beam by a direct scalar product. The direction vectors are mediated via the tensor $\mathbb{1}_\perp$ which reflects the intermediate light propagation in the two eliminated modes. The parameters in Eqs. (S9) are defined as

$$\begin{aligned}
\Omega &= \frac{\sqrt{2\kappa_R}a_{in}}{\kappa + i\Delta_c}\,,\\
\delta_{LS} &= -\frac{\Delta_c}{\kappa^2 + \Delta_c^2}\,,\\
\zeta_S &= \frac{\kappa}{\kappa^2 + \Delta_c^2}\,.
\end{aligned} \tag{S10}$$

## REFLECTIVITY

Experiments can determine the reflected (or transmitted) intensity $|R|^2$ ($|T|^2$) on the thin-film cavity. The reflection coefficient $R$ is given by $R = \langle a_{out}\rangle / a_{in}$ with the output field operator $a_{out}$ defined as

$$a_{out} = -a_{in}(\hat{a}_{out}^{*}\cdot\hat{a}_{in}) + \sqrt{2\kappa_R}[(\hat{a}_{out}^{*}\cdot\hat{a}_1)a_1 + (\hat{a}_{out}^{*}\cdot\hat{a}_2)a_2]\,. \tag{S11}$$

Using the expressions and quantities above, the reflection coefficient can be written as

$$\begin{aligned} R &= \left(\frac{2\kappa_R}{\kappa+i\Delta_c}-1\right)\hat{a}^*_{out}\cdot\hat{a}_{in} \\ &- \frac{i}{a_{in}}\frac{\sqrt{2\kappa_R}}{\kappa+i\Delta_c}\sum_\mu(\hat{a}^*_{out}\cdot\mathbb{1}_\perp\cdot\hat{d}_\mu)c_\mu\sqrt{N_\mu}g^*\langle E_\mu|\rho|G\rangle\,. \end{aligned} \tag{S12}$$

## EXPRESSIONS FOR COHERENCE TERMS

From Eq. (S8), the sum of the two relevant coherence terms can be written as

$$\rho_{23}+\rho_{13}=\frac{i\sqrt{\frac{16}{3}}g\sqrt{N}\Omega(\gamma-2i\Delta)}{(\gamma-2i\Delta)(\gamma'-2i\Delta')+(2\phi)^2}\,, \tag{S13}$$

where $\gamma'=\gamma+\frac{4}{3}|g|^2N\zeta_S$ , $\Delta'=\Delta-\frac{2}{3}|g|^2N\delta_{LS}$ and $\phi=\frac{1}{2}(\delta_g+\delta_e)$. Here $\gamma$ is the nuclear spontaneous decay rate and $\delta_g$ ($\delta_e$) denotes the energy difference between two adjacent ground (excited) sub-states. Next, we consider the resonant case ( $\Delta_c=0$) in which $\delta_{LS}=0$. Then we obtain

$$\rho_{23}+\rho_{13}=\frac{i\sqrt{\frac{16}{3}}g\sqrt{N}\Omega(\gamma-2i\Delta)}{(\gamma-2i\Delta)(\gamma'-2i\Delta)+(2\phi)^2}\,. \tag{S14}$$

With $\gamma'\gg\gamma$, the expression of the coherence $\rho_{21}+\rho_{31}$ is very similar to the EIT case, as discussed in the following Section. To obtain the reflectivity spectra numerically, we set up the cavity consisting of a Pd(5nm)/C(40nm)/Pd(30nm) layer system with Pd layers acting as mirrors and C as guiding layer. A 1 nm thick $^{57}$Fe layer is placed in the center of the carbon layer. An external magnetic field of 6.4 T is applied, leading to the hyperfine splitting $\phi=6\gamma$. The numerical results obtained are compared with CONUSS [49] simulations in Fig. 2 in the main text. The parameters used in the quantum model described above are $\kappa_R=312310\gamma$, $\kappa=456250\gamma$ and $\sqrt{N}|g|=\sqrt{6300000}\gamma$. We investigate the resonant case $\Delta_c=0$. In this case, the collective decay rate $\gamma'=\gamma+\frac{4}{3}|g|^2N\zeta_S=19.4\gamma$.

## COMPARISON WITH TRADITIONAL EIT IN A $\Lambda$ THREE-LEVEL SYSTEM

Traditional EIT in atomic media occurs in a $\Lambda$ three-level system with an upper state $|a\rangle$ and two ground states $|b\rangle$ and $|c\rangle$. Initially the atoms are all in the ground state $|b\rangle$ and we assume

that the control field is resonant with the transition $|c\rangle \to |a\rangle$. The coherence between state $|a\rangle$ and state $|b\rangle$ is given by [44]:

$$\rho_{ab} = \frac{i\Omega_p(\Gamma_{bc} + i\delta_p)}{(\Gamma_{ab} + i\delta_p)(\Gamma_{bc} + i\delta_p) + \Omega_c^2/4}, \tag{S15}$$

where $\delta_p$ is the detuning between the resonant frequency of transition $|b\rangle \to |a\rangle$ and the probe pulse, and $\Gamma_{ab}$ and $\Gamma_{bc}$ are dephasing rates for the $|b\rangle \to |a\rangle$ and $|b\rangle \to |c\rangle$ transitions, respectively. Typically, a condition for EIT is that $\Gamma_{ab} \gg \Gamma_{bc}$. Moreover, $\Omega_p$ is the Rabi frequency of the probe pulse and $\Omega_c$ is the Rabi frequency of the control field. We note here that the structure of the expression above is identical to the one presented in Eq. (S14).

The coherence as a function of the complex variable $\delta_p$ has two poles [48],

$$\delta_\pm = \frac{1}{2}\left(i\Gamma_{ab} + i\Gamma_{bc} \pm \sqrt{\Omega_c^2 - (\Gamma_{ab} + \Gamma_{bc})^2}\right). \tag{S16}$$

Then the coherence $\rho_{ab}$ can be presented as a superposition of two resonant responses associated with the transitions from the ground state to the corresponding decaying dressed states [48]:

$$\rho_{ab} = \frac{\Omega_p A_+}{\delta_p - \delta_+} + \frac{\Omega_p A_-}{\delta_p - \delta_-}, \tag{S17}$$

where $A_\pm$ are defined as

$$A_\pm = \pm\frac{\delta_\pm - i\Gamma_{bc}}{\delta_+ - \delta_-}. \tag{S18}$$

Thus, the control field splits the upper level $|a\rangle$ and the probe pulse drives both transitions between ground state $|b\rangle$ and the two split upper levels. The interference between the two transitions results in the characteristic feature of EIT in the range of the control field intensities $4\Gamma_{ab}\Gamma_{bc} \le \Omega_c^2 < 4(\Gamma_{ab} - \Gamma_{bc})^2$ [48]. In the thin film x-ray cavity system, the EIT-like effect occurs due to the interference between the two $\Delta m = 0$ transitions under the presence of vacuum-mediated coupling between the two upper states. The splitting of the excited states in the two systems depicted are generated by the strong control field and the magnetic field, respectively.

## MAXWELL-BLOCH PROPAGATION EQUATION FOR X-RAYS

Finally we pursue an analytical description of the pulse propagation through the nuclear cavity medium. The evolution of the Heisenberg operator corresponding to the x-ray field can be described in a slowly varying amplitude approximation by the propagation equation [28]

$$\left(\frac{\partial}{\partial t} + c\frac{\partial}{\partial z}\right)\Omega(z,t) = ig\sqrt{\frac{1}{3}N}[\rho_{31}(z,t) + \rho_{32}(z,t)]. \tag{S19}$$

The evolution of the coherences are described by the Heisenberg equations

$$\begin{aligned}\frac{\partial(\rho_{31}+\rho_{32})}{\partial t} &= i\sqrt{\frac{4}{3}}Ng\Omega-\left(\frac{\gamma'}{2}+i\Delta\right)(\rho_{31}+\rho_{32}) \\ &\quad -i\phi(\rho_{31}-\rho_{32}), \\ \frac{\partial(\rho_{31}-\rho_{32})}{\partial t} &= -\left(\frac{\gamma}{2}+i\Delta\right)(\rho_{31}-\rho_{32})-i\phi(\rho_{31}+\rho_{32}).\end{aligned} \tag{S20}$$

Disregarding the slow decay $\gamma$, we may derive

$$\begin{aligned}\rho_{31}+\rho_{32} &= \frac{i}{\phi}\frac{\partial(\rho_{31}-\rho_{32})}{\partial t}, \\ \rho_{31}-\rho_{32} &= \frac{\sqrt{\frac{4}{3}Ng\Omega}}{\phi}+\frac{i}{\phi}\left(\frac{\gamma'}{2}+\frac{\partial}{\partial t}\right)\left[\frac{i}{\phi}\frac{\partial(\rho_{31}-\rho_{32})}{\partial t}\right].\end{aligned} \tag{S21}$$

The change of the hyperfine magnetic field leads to a time-dependent function $\phi(t)$. We assume a sufficiently slow change of $\phi(t)$ and simplify the equations using adiabatic conditions. In this limit,

$$\rho_{31}(z,t)-\rho_{32}(z,t)=\frac{\sqrt{\frac{4}{3}Ng\Omega(z,t)}}{\phi(t)}. \tag{S22}$$

Finally we achieve the propagation equation of the x-ray pulse in the perturbative and the adiabatic limit [Eq. (3) in the main text]

$$\left(\frac{\partial}{\partial t}+c\frac{\partial}{\partial z}\right)\Omega(z,t)=-\frac{2g^2N}{3\phi(t)}\frac{\partial}{\partial t}\frac{\Omega(z,t)}{\phi(t)}, \tag{S23}$$

which allows the identification of a dark state polariton and reveals control mechanisms over the x-ray pulse propagation.
